# Supplementary material for: Energy-Efficient Transmission Scheduling with Strict Underflow Constraints
Source: arXiv:0908.1774 source file (2010-02-16)
Supplement: Supplementary file 1 [file appendix_structure_inf_average_proof.tex]

What to show:
\begin{itemize}
\item Conditions general, W, B of Schal
\item Assumption 5.5.1 of Hernandez-Lerma book (using convexity-type argument from Fernandez paper)
\end{itemize}

First two give me ACOE, optimality of selector that satisfies ACOE, $\rho^*$ as limit $\alpha$ to 1 (Schal), $\rho^*$ is constant average cost, sequence that w's converge by Theorem 5.5.4 of H-L, policy convergence as described in (ii) of Schal\cite{schal2}

structure follows from convexity, supermodularity of w, as any policy satisfying ACOE is average cost optimal

Extra:
\begin{itemize}
\item limit $\alpha$ to 1 of w's exists (w nondecreasing in $\alpha$, bounded above)
\item limit $\alpha$ to 1 of selectors exists ($b_{\infty,k,\alpha}$ nondecreasing in $\alpha$ and bound independent of $\alpha$)
\item triplet of $\rho^*$, w, selector satisfy ACOE (follows from last part of Theorem 5.5.4 by showing triplet satisfies ACOE - every term in reorganized DCOE converges)
\end{itemize}

%What to show:
%\begin{itemize}
%\item Conditions general, W, B of Schal
%\item Assumption 5.5.1 of H-L (using convexity-type argument)
%\end{itemize}
%
%First two give me ACOE, optimality of selector, $\rho^*$ as limit $\alpha$ to 1, $\rho^*$ is constant average cost, sequence that w's converge by Theorem 5.5.4 of H-L. Policy convergence as described in (ii) of Schal\cite{schal2}
%
%Extra:
%\begin{itemize}
%\item limit $\alpha$ to 1 of w's exists (monotonic in $\alpha$, finite)
%\item limit $\alpha$ to 1 of selectors exists ($b_{\infty,k,\alpha}$ nondecreasing in $\alpha$ and bound independent of $\alpha$)
%\item triplet of $rho^*$, w, selector satisfied ACOE (follows from last part of Theorem 5.5.4 by showing triplet satisfies ACOE)
%\end{itemize}

The following two lemmas are similar in spirit to the analysis of the deterministic piecewise-linear ordering cost, random demand inventory model in \cite{zahrn}.
\begin{lemma} \label{Le:wmon}
$w_{\infty,\alpha}(\textbf{x},\textbf{s})$ is nondecreasing in $\alpha$ for all $\textbf{x} \in {\cal X}$ and $\textbf{s} \in {\cal S}$.
\end{lemma}
\begin{proof}
cc
\end{proof}
From Condition (B) and Lemma \ref{Le:wmon}, we conclude $w_{\infty,1}(\textbf{x},\textbf{s}):=\lim\limits_{\alpha \nearrow 1}w_{\infty,\alpha}(\textbf{x},\textbf{s})$ exists and is finite for all $\textbf{x} \in {\cal X}$ and $\textbf{s} \in {\cal S}$. 

\begin{lemma} \label{Le:bmon}
For every $k \in \{-1,0,1,\ldots,K\}$ and $s \in {\cal S}$, the critical numbers $b_{\infty,k,\alpha}(s)$ defined in (d) of Theorem \ref{Th:two:infd} are nondecreasing in $\alpha$. Moreover, there exists a bounding function $\hat{\kappa}(k,s)$ such that $b_{\infty,k,\alpha}(s)\leq\hat{\kappa}(k,s)$ for all $\alpha \in [0,1)$.
\end{lemma}
\begin{proof}
cc
\end{proof}
